# Supplementary material for: Reinforcement Learning for Multi-Objective Multi-Echelon Supply Chain Optimisation
Source: arXiv:2507.19788 source file (2025-07-26)
Supplement: Supplementary file 1 [file __Suplementary_Material.tex]

%% 
%% Copyright 2019-2024 Elsevier Ltd
%% 
%% This file is part of the 'CAS Bundle'.
%% --------------------------------------
%% 
%% It may be distributed under the conditions of the LaTeX Project Public
%% License, either version 1.3c of this license or (at your option) any
%% later version.  The latest version of this license is in
%%    http://www.latex-project.org/lppl.txt
%% and version 1.3c or later is part of all distributions of LaTeX
%% version 1999/12/01 or later.
%% 
%% The list of all files belonging to the 'CAS Bundle' is
%% given in the file `manifest.txt'.
%% 
%% Template article for cas-sc documentclass for 
%% double column output.

\documentclass[a4paper,fleqn]{cas-sc}

% If the frontmatter runs over more than one page
% use the longmktitle option.

%\documentclass[a4paper,fleqn,longmktitle]{cas-sc}

%\usepackage[numbers]{natbib}
%\usepackage[authoryear]{natbib}
\usepackage{natbib}
\usepackage{graphicx}
\usepackage{soul}
\usepackage{comment}
\usepackage{xcolor}
\usepackage{booktabs}
\usepackage{amssymb}
\usepackage{multirow}
\usepackage{cite}
\usepackage{amsmath}
\usepackage{amsfonts}
\usepackage{algorithmic}
\usepackage{array}
\usepackage{stfloats}
\usepackage{tabularx}
\usepackage{float}
\usepackage{subcaption}
\usepackage{subfig}
\usepackage{setspace}
\usepackage{float}
% Redefine \url command to do nothing

%%%Author macros
\def\tsc#1{\csdef{#1}{\textsc{\lowercase{#1}}\xspace}}
\tsc{WGM}
\tsc{QE}
%%%

% Uncomment and use as if needed
%\newtheorem{theorem}{Theorem}
%\newtheorem{lemma}[theorem]{Lemma}
%\newdefinition{rmk}{Remark}
%\newproof{pf}{Proof}
%\newproof{pot}{Proof of Theorem \ref{thm}}
\newif\ifcomment
\commentfalse  % disables the block
% \commenttrue  % enables the block
\begin{document}
\let\WriteBookmarks\relax
\def\floatpagepagefraction{1}
\def\textpagefraction{.001}

\newpage % Ensures the following content starts on a new page

% Short title
\shorttitle{RL for MO and ME Supply Chain Optimisation}    

% Short author
\shortauthors{R.M. Rachman et~al.}  

% Main title of the paper
\title [mode = title]{Reinforcement Learning for Multi-Objective and Multi-Echelon Supply Chain Optimisation}  

% Title footnote mark
% eg: \tnotemark[1]
\tnotemark[1] 

% Title footnote 1.
% eg: \tnotetext[1]{Title footnote text}
\tnotetext[1]{This document is the results of the research
   project funded by UK Research and Innovation, University of Manchester, and Peak.} 

% First author
%
% Options: Use if required
% eg: \author[1,3]{Author Name}[type=editor,
%       style=chinese,
%       auid=000,
%       bioid=1,
%       prefix=Sir,
%       orcid=0000-0000-0000-0000,
%       facebook=<facebook id>,
%       twitter=<twitter id>,
%       linkedin=<linkedin id>,
%       gplus=<gplus id>]

\author[1]{R.M. Rachman}%[<options>]

% Corresponding author indication
\cormark[1]

% Footnote of the first author
\fnmark[1]

% Email id of the first author
\ead{rifny.rachman@postgrad.manchester.ac.uk}

% URL of the first author
%\ead[url]{}

% Credit authorship
% eg: \credit{Conceptualization of this study, Methodology, Software}
\credit{Conceptualisation, Software, Methodology, Formal analysis, Writing - original draft}

% Address/affiliation
\affiliation[1]{organization={The University of Manchester},
            addressline={Oxford Road}, 
            city={Manchester},
%          citysep={}, % Uncomment if no comma needed between city and postcode
            postcode={M13 9PL}, 
            %state={},
            country={United Kingdom}}

\author[2]{J. Tingey}%[]

% Footnote of the second author
%\fnmark[2]

% Email id of the second author
\ead{josh.tingey@peak.ai}

% URL of the second author
%\ead[url]{}

% Credit authorship
\credit{Conceptualisation, Software, Resources, Validation}

% Address/affiliation
\affiliation[2]{organization={Peak AI, Ltd},
            %addressline={}, 
            city={Manchester},
%          citysep={}, % Uncomment if no comma needed between city and postcode
            %postcode={}, 
            %state={},
            country={United Kingdom}}

% Corresponding author text
\cortext[1]{Corresponding author}

\author[1]{R. Allmendinger}
\ead{richard.allmendinger@manchester.ac.uk}
\credit{Conceptualisation, Writing - review \& editing, Supervision, Validation}

\author[1]{P. Shukla}
\ead{pradyumn.shukla@manchester.ac.uk}
\credit{Writing - review \& editing, Supervision, Validation}

\author[1]{W. Pan}
\ead{wei.pan@manchester.ac.uk}
\credit{Writing - review \& editing, Supervision, Validation}
% Footnote text
%\fntext[1]{}

% For a title note without a number/mark
%\nonumnote{}

%\maketitle
\onehalfspacing
% Main text

% Numbered list
% Use the style of numbering in square brackets.
% If nothing is used, default style will be taken.
%\begin{enumerate}[a)]
%\item 
%\item 
%\item 
%\end{enumerate}  

% Unnumbered list
%\begin{itemize}
%\item 
%\item 
%\item 
%\end{itemize}  

% Description list
%\begin{description}
%\item[]
%\item[] 
%\item[] 
%\end{description}  

% Uncomment and use as the case may be
%\begin{theorem} 
%\end{theorem}

% Uncomment and use as the case may be
%\begin{lemma} 
%\end{lemma}

%% The Appendices part is started with the command \appendix;
%% appendix sections are then done as normal sections
%% \appendix

% To print the credit authorship contribution details
%\printcredits
\clearpage
\section{Pareto Front Sets from All Runs}\label{appendix}
\begin{figure}[htbp!]
    \centering
    \begin{subfigure}{0.32\textwidth}
        \includegraphics[width=\textwidth]{pf_simple_3d-1_v2.PNG}
        \caption{first 3D view-Simple SC}
    \end{subfigure}
    \hfill
    \begin{subfigure}{0.32\textwidth}
        \includegraphics[width=\textwidth]{pf_simple_3d-2_v2.PNG}
        \caption{second 3D view-Simple SC}
    \end{subfigure}
    \hfill
    \begin{subfigure}{0.32\textwidth}
        \includegraphics[width=\textwidth]{pf_simple_3d-3_v2.PNG}
        \caption{third 3D view-Simple SC}
    \end{subfigure}
    
    %\vskip\baselineskip 
    \begin{subfigure}{0.32\textwidth}
        \includegraphics[width=\textwidth]{pf_moderate_3d-1_v2.PNG}
        \caption{first 3D view-Moderate SC}
    \end{subfigure}   
    \hfill
    \begin{subfigure}{0.32\textwidth}
        \includegraphics[width=\textwidth]{pf_moderate_3d-2_v2.PNG}
        \caption{second 3D view-Moderate SC}
    \end{subfigure}
    \hfill
    \begin{subfigure}{0.32\textwidth}
        \includegraphics[width=\textwidth]{pf_moderate_3d-3_v2.PNG}
        \caption{third 3D view-Moderate SC}
    \end{subfigure}

    \begin{subfigure}{0.32\textwidth}
        \includegraphics[width=\textwidth]{pf_all_complex_3d-1_v2.PNG}
        \caption{first 3D view-Complex SC}
    \end{subfigure}   
    \hfill
    \begin{subfigure}{0.32\textwidth}
        \includegraphics[width=\textwidth]{pf_all_complex_3d-2_v2.PNG}
        \caption{second 3D view-Complex SC}
    \end{subfigure}
    \hfill
    \begin{subfigure}{0.32\textwidth}
        \includegraphics[width=\textwidth]{pf_all_complex_3d-3_v2.PNG}
        \caption{third 3D view-Complex SC}
    \end{subfigure}
    \caption{Scatter plots of all resulting PF sets from all algorithms across 810 runs in total: (3 problems x 21 weights x 10 runs) of PPO, (3 problems x 4 scenarios x 10 runs) of MORL/D, and (3 problems x 20 runs) of NSGA-II. The plot shows all non-dominated solutions from PPO, each scenario of MORL/D, and NSGA-II except The plot shows that all results are within approximately similar objective space.}
    \label{fig:pf_all_all}
\end{figure}
\clearpage
\section{Parameters for Experimentation}   
\begin{minipage}{\textwidth}  % Full width of the page
    \centering
    \small    
    \subsection{Simple SC}% First table
    \captionof{table}{\small Node parameter values that correspond to the facilities in Simple SC environment.}
    \label{tab:para_value}
    \begin{tabularx}{9cm}{ccccccc}
        \toprule
        Node & $I_{0j}$ & $c_j^\varsigma$ & $e^\varsigma_j$ & $c_k^\psi$ & $v_k^\psi$ & $e^\psi_k$ \\
        \midrule
        3 & 380 & 0.1100 & 0.0002 & 2.0000 & 1.0000 & 5.0126\\
        4 & 350 & 0.1300 & 0.0002 & 2.2000 & 1.0000 & 4.5754\\
        5 & 400 & 0.1200 & 0.0002 & NA & NA & NA\\
        6 & 80 & 0.1500 & 0.0002 & NA & NA & NA\\
        \bottomrule      
    \end{tabularx}

    % Second table
    \captionof{table}{\small Transport parameter values that correspond to product delivery.}
    \label{tab:trans_value}
    \begin{tabularx}{7cm}{cccc}
        \toprule
        From Node & To Node & $c^\tau_{ij}$ & $e^\tau_{ij}$ \\
        \midrule
        \multirow{2}{*}{1} & 2 & 0.2200 & 0.1258\\
        & 3 & 0.6900 & 0.3947\\
        \hline
        \multirow{2}{*}{2} & 4 & 1.0550 & 0.6035\\
        & 5 & 0.4300 & 0.2460\\
        \hline
        \multirow{2}{*}{3} & 4 & 0.4850 & 0.2774\\
        & 5 & 0.7500 & 0.4290\\
        \bottomrule
    \end{tabularx}
    \subsection{Moderate SC}
    \captionof{table}{\small Node parameter values that correspond to the facilities in Moderate SC environment.}
    \label{tab:para_value}
    \begin{tabularx}{9cm}{ccccccc}
        \toprule
        Node & $I_{0j}$ & $c_j^\varsigma$ & $e^\varsigma_j$ & $c_k^\psi$ & $v_k^\psi$ & $e^\psi_k$ \\
        \midrule
        3 & 380 & 0.1100 & 0.0002 & 2.0000 & 1.0000 & 5.0126\\
        4 & 350 & 0.1300 & 0.0002 & 2.2000 & 1.0000 & 4.5754\\
        5 & 400 & 0.1200 & 0.0002 & 2.3000 & 1.0000 & 5.4491\\
        6 & 80 & 0.1500 & 0.0002 & NA & NA & NA\\
        7 & 110 & 0.2000 & 0.0002 & NA & NA & NA\\
        8 & 100 & 0.2500 & 0.0002 & NA & NA & NA\\
        9 & 80 & 0.3000 & 0.0002 & NA & NA & NA\\
        10 & 120 & 0.2000 & 0.0002 & NA & NA & NA\\
        \bottomrule      
    \end{tabularx}

\end{minipage}

\begin{minipage}{\textwidth}  % Full width of the page
    \centering
    \small    
    % First table

    \vspace{0.5cm}  % Adjust space between the tables as needed

    % Second table
    \captionof{table}{\small Transport parameter values that correspond to product delivery.}
    \label{tab:trans_value}
    \begin{tabularx}{7cm}{cccc}
        \toprule
        From Node & To Node & $c^\tau_{ij}$ & $e^\tau_{ij}$ \\
        \midrule
        \multirow{3}{*}{1} & 3 & 0.2200 & 0.1258\\
        & 4 & 0.6900 & 0.3947\\
        & 5 & 0.5650 & 0.3232\\
        \hline
        \multirow{3}{*}{2} & 3 & 1.0550 & 0.6035\\
        & 4 & 0.6500 & 0.3718\\
        & 5 & 0.6300 & 0.3604\\
        \hline
        \multirow{2}{*}{3} & 6 & 0.0750 & 0.0429\\
        & 7 & 0.4300 & 0.2460\\
        \hline
        \multirow{2}{*}{4} & 6 & 0.6300 & 0.3604\\
        & 7 & 0.2300 & 0.1316\\
        \hline
        \multirow{2}{*}{5} & 6 & 0.4950 & 0.2831\\
        & 7 & 0.0750 & 0.0429\\
        \hline
        \multirow{3}{*}{6} & 8 & 1.0950 & 0.6263 \\
        & 9 & 0.6250 & 0.3575\\
        & 10 & 0.9500 & 0.5434\\
        \hline
        \multirow{3}{*}{7} & 8 & 1.6400 & 0.9381\\
        & 9 & 1.1600 & 0.6635\\
        & 10 & 0.5800 & 0.3318\\
        \bottomrule
    \end{tabularx}
    \subsection{Complex SC}
    \captionof{table}{\small Node parameter values that correspond to the facilities in Complex SC environment.}
    \label{tab:para_value}
    \begin{tabularx}{9cm}{ccccccc}
        \toprule
        Node & $I_{0j}$ & $c_j^\varsigma$ & $e^\varsigma_j$ & $c_k^\psi$ & $v_k^\psi$ & $e^\psi_k$ \\
        \midrule
        4 & 155 & 0.2300 & 0.0002 & 2.0000 & 1.0000 & 5.0126\\
        5 & 267 & 0.3500 & 0.0002 & 2.2000 & 1.0000 & 4.5754\\
        6 & 342 & 0.2200 & 0.0002 & 2.1000 & 1.0000 & 5.4491\\
        7 & 211 & 0.1100 & 0.0002 & 2.0000 & 1.0000 & 6.1232\\
        8 & 162 & 0.2900 & 0.0002 & 2.3000 & 1.0000 & 5.5157\\
        9 & 195 & 0.3700 & 0.0002 & NA & NA & NA\\
        10 & 333 & 0.1100 & 0.0002 & NA & NA & NA\\
        11 & 96 & 0.3600 & 0.0002 & NA & NA & NA\\
        12 & 285 & 0.3300 & 0.0002 & NA & NA & NA\\
        13 & 68 & 0.2600 & 0.0002 & NA & NA & NA\\
        14 & 379 & 0.3000 & 0.0002 & NA & NA & NA\\
        15 & 344 & 0.1700 & 0.0002 & NA & NA & NA\\
        16 & 66 & 0.2900 & 0.0002 & NA & NA & NA\\
        17 & 356 & 0.2700 & 0.0002 & NA & NA & NA\\
        18 & 382 & 0.2300 & 0.0002 & NA & NA & NA\\
        19 & 362 & 0.3700 & 0.0002 & NA & NA & NA\\
        \bottomrule      
    \end{tabularx}
\end{minipage}

\begin{table}
    \centering
    \caption{Transport parameter values that correspond to product delivery.}
    \label{tab:trans_value}
    \begin{minipage}[t]{0.45\textwidth}  % First half of the table
        \centering
        \small
        \begin{tabularx}{\textwidth}{cccc}
            \toprule
            From Node & To Node & $c^\tau_{ij}$ & $e^\tau_{ij}$ \\
            \midrule
            \multirow{5}{*}{1} & 4 & 0.5350 & 0.3060\\
            & 5 & 0.2650 & 0.1516\\
            & 6 & 1.8450 & 1.0553\\
            & 7 & 1.6000 & 0.9152\\
            & 8 & 1.4400 & 0.8237\\
            \hline
            \multirow{5}{*}{2} & 4 & 0.3600 & 0.2059\\
            & 5 & 0.2950 & 0.1687\\
            & 6 & 1.2350 & 0.7064\\
            & 7 & 0.6250 & 0.3575\\
            & 8 & 1.8550 & 1.0611\\
            \hline
            \multirow{5}{*}{3} & 4 & 0.6000 & 0.3432\\
            & 5 & 0.1750 & 0.1001\\
            & 6 & 0.7450 & 0.4261\\
            & 7 & 1.3300 & 0.7608\\
            & 8 & 0.1700 & 0.0972\\
            \hline
            \multirow{3}{*}{4} & 9 & 1.9900 & 1.1383\\
            & 10 & 0.3400 & 0.1945\\
            & 11 & 0.8100 & 0.4633\\
            \hline
            \multirow{3}{*}{5} & 9 & 1.5150 & 0.8666\\
            & 10 & 0.6600 & 0.3775\\
            & 11 & 0.6450 & 0.3689\\
            \hline
            \multirow{3}{*}{6} & 9 & 1.6950 & 0.9695\\
            & 10 & 1.5800 & 0.9038\\
            & 11 & 0.8150 & 0.4662\\
            \bottomrule
            \multirow{5}{*}{ }\\
            \\
            \\
            \\
            \\
        \end{tabularx}
    \end{minipage}%
    \hspace{0.02\textwidth}  % Space between the two tables
    \begin{minipage}[t]{0.45\textwidth}  % Second half of the table
        \centering
        \small
        \begin{tabularx}{\textwidth}{cccc}
            \toprule
            From Node & To Node & $c^\tau_{ij}$ & $e^\tau_{ij}$ \\
            \midrule
            \multirow{3}{*}{7} & 9 & 1.6150 & 0.9238\\
            & 10 & 1.2600 & 0.7207\\
            & 11 & 0.6750 & 0.3861\\
            \hline
            \multirow{3}{*}{8} & 9 & 1.0300 & 0.5892\\
            & 10 & 1.0900 & 0.6235\\
            & 11 & 1.6300 & 0.9324\\
            \hline
            \multirow{3}{*}{9} & 12 & 1.9650 & 1.1240 \\
            & 13 & 1.9250 & 1.1011\\
            & 14 & 1.6200 & 0.9266\\
            \hline
            \multirow{3}{*}{10} & 8 & 1.4900 & 0.8523\\
            & 9 & 1.9600 & 1.1211\\
            & 10 & 0.6350 & 0.3632\\
            \hline
            \multirow{3}{*}{11} & 8 & 1.8700 & 1.0696\\
            & 9 & 0.2000 & 0.1144\\
            & 10 & 1.8550 & 1.0611\\
            \hline
            \multirow{5}{*}{12} & 15 & 1.9450 & 1.1125\\
            & 16 & 0.9650 & 0.5520\\
            & 17 & 1.9050 & 1.0897\\
            & 18 & 0.9000 & 0.5148\\
            & 19 & 0.6900 & 0.3947\\
            \hline
            \multirow{5}{*}{13} & 15 & 0.8050 & 0.4605\\
            & 16 & 1.0650 & 0.6092\\
            & 17 & 1.8400 & 1.0525\\
            & 18 & 0.8300 & 0.4748\\
            & 19 & 1.8850 & 1.0782\\
            \hline
            \multirow{5}{*}{14} & 15 & 1.6600 & 0.9495\\
            & 16 & 1.5100 & 0.8637\\
            & 17 & 0.5900 & 0.3375\\
            & 18 & 0.4000 & 0.2288\\
            & 19 & 1.3950 & 0.7979\\
            \bottomrule
        \end{tabularx}
    \end{minipage}
\end{table}

\ifcomment
\section{Hyperparameters for Experimentation}
\begin{minipage}{\textwidth}
    \centering
    \small   
    \captionof{table}{\small Hyperparameters of NSGA-II to solve the SC problem.}
    \label{tab:nsga_parameters}
    \begin{tabularx}{7cm}{ll}
        \toprule
        Hyperparameters & Values\\
        \midrule
        Population size & 300\\
        Offspring number & 30\\
        Cross-over operator & binary (SBX)\\
        Cross-over probability & 90\%\\
        Cross-over $\eta$ & 15\\
        Mutation method & polynomial\\
        Mutation $\eta$ & 20\\
        \bottomrule
    \end{tabularx}
\end{minipage}

\begin{table}[h]
    \centering
    \begin{minipage}{0.48\textwidth}  % First half of the page for the PPO table
        \centering
        \captionof{table}{\small Hyperparameters of PPO Algorithm}
        \label{tab:hyperparameter_ppo}
        \begin{tabularx}{\textwidth}{ll}
            \toprule
            Hyperparameters & Values \\
            \midrule
            Learning rate & 3 x $10^{-4}$ \\
            Number of steps & 2048 \\
            Minibatch size & 64 \\
            Number of epochs & 10 \\
            Discount factor & 0.99 \\
            GAE Weight & 0.95 \\
            Clipping range & 0.2 \\
            Entropy coefficient & 0 \\
            Value function coefficient for loss & 0.5 \\
            Maximum gradient clipping & 0.5 \\
            Episode per iteration & 50 \\
            Steps per episode & 100 \\
            Total time steps & 5 x $10^{5}$ \\
            Neural network activation function & Tanh \\
            \bottomrule
        \end{tabularx}
    \end{minipage}%
    \hspace{0.04\textwidth}  % Space between tables
    \begin{minipage}{0.48\textwidth}  % Second half of the page for the MORL/D table
        \centering
        \captionof{table}{\small Hyperparameters of MORL/D Algorithm with MOSAC Policy}
        \label{tab:hyperparameter_MORLD}
        \begin{tabularx}{\textwidth}{ll}
            \toprule
            Hyperparameters & Values \\
            \midrule
            \textbf{MORL/D} & \\
            Discount factor & 0.995 \\
            Population size & 6 \\
            Exchange every & 5 x $10^4$ \\
            Total time steps & 5 x $10^5$ \\
            Neighbourhood size & 1 \\
            Update passes & 10 \\
            Initial weight distribution & uniform \\
            \midrule
            \textbf{MOSAC} & \\
            Buffer size & $10^6$ \\
            Discount factor & 0.99 \\
            Target smoothing coefficient & 0.005 \\
            Batch size & 128 \\
            Steps before learning & $10^3$ \\
            Hidden neurons & [256;256] \\
            Actor learning rate & 3 x $10^{-4}$ \\
            Critic learning rate & $10^{-3}$ \\
            Actor training frequency & 2 \\
            Target training frequency & 1 \\
            Activation function & ReLU \\
            \bottomrule
        \end{tabularx}
    \end{minipage}
\end{table}
\fi
\newpage
%% Loading bibliography style file
%\bibliographystyle{model1-num-names}

% Biography
%\bio{}
% Here goes the biography details.
%\endbio

%\bio{pic1}
% Here goes the biography details.
%\endbio

\end{document}
